# Supplementary material for: HouseDiffusion: Vector Floorplan Generation via a Diffusion Model with Discrete and Continuous Denoising
Source: arXiv:2211.13287 source file (2022-11-23)
Supplement: Supplementary file 1 [file appendix.tex]

%\newpage
The supplementary document provides 1) ablation studies on the hyperparameters (e.g., the number of steps and the target output of the model); 2) more experimental results on the non-manhattan RPLAN dataset; 3) more analysis on our discrete denoising and AnalogBits~\cite{chen2022analog}; and 4) 
%, including the effect of number of steps and the target output for the model. 
%In addition, we provide more details of our non-manhattan version of RPLAN as we as more analysis on Discrete prediction and AnalogBits~\cite{chen2022analog}. Finally, we arrange 
additional qualitative examples of our system and competing methods. 
%method compared with the baseline.
Please also see the supplementary video for more examples.

%The supplementary document provides ablation studies on the hyperparameters (e.g., the number of steps and the target output of the model).
%, including the effect of number of steps and the target output for the model. 
%In addition, we provide more details of our non-manhattan version of RPLAN as we as more analysis on Discrete prediction and AnalogBits~\cite{chen2022analog}. Finally, we arrange additional qualitative examples of our method compared with the baseline. Please see the attached video in our supplementary for more examples.

\section{Diffusion Hyperparameters}
%on Diffusion Hyperparameters}
\mysubsubsection{Target output}
\label{sec:target_output}
In the diffusion process, we can train the network to predict either $x_0$ or $\epsilon$. While both options are mathematically similar,
%can be mapped to each other,
we found that training to predict $\epsilon$ works better.
%for the network in our task.
Table~\ref{tab:output_value} shows the results. This is because directly predicting the final coordinates ($x_0$) in the early reverse steps is a lot more challenging than predicting the per-step noise $\epsilon$.
% We hypothesize that this is due to the hardness of the task.
%as directly predicting the corners' coordinates in $x_0$ in the first steps of denoising is a more challenging task while predicting $\epsilon$ in each step breaks down the task into smaller steps.
%
We can see the same pattern in overfitting on a single data when the network can learn significantly faster when predicting $x_0$ comparing to $\epsilon$, and we found it also consistent with the results of AnalogBits~\cite{chen2022analog} when comparing the results on \textsc{Cifar-10} and \textsc{ImageNet} datasets.
\begin{table}[b]
\caption{Training the network to predict $\epsilon$ works better in our task comparing with $x_0$ as the output of the model in each step.}
\vspace{-1em}
\label{tab:output_value}
\centering
\setlength{\tabcolsep}{3pt}
\small
\scalebox{1.}{\begin{tabular}{c|c|c}
\toprule
   Network's output & Diversity $(\downarrow)$ & Compatibility $(\downarrow)$\\
    \cmidrule(lr){1-1}\cmidrule(lr){2-2} \cmidrule(lr){3-3}
    $x_0$ & 121.2\scalebox{0.8}{$\pm$1.9} & 4.2\scalebox{0.8}{$\pm$0.0} \\
    \midrule
    $\epsilon$ & 38.8\scalebox{0.8}{$\pm$0.9} & 2.2\scalebox{0.8}{$\pm$0.0}\\
    \bottomrule
\end{tabular}}
\end{table}

%%%%%%
\mysubsubsection{Number of steps and the noise schedule}
\label{sec:dm_hyperparams}
Table~\ref{tab:dm_params} shows the sensitivity of our method to the noise schedule and the number of steps. Using a smaller number of steps leads to larger jumps between different time steps, which is harder to predict for the model, and using a larger number of steps needs more capacity to learn the distribution states of all steps. Similarly, using the cosine schedule proposed by Nichol and Dhariwal\cite{nichol2021improved} works better by preventing abrupt changes comparing the Linear schedule proposed by Ho et al.~\cite{ho2020denoising}.
\begin{table}[tb]
\caption{Results of hyper-parameter tuning on the number of steps and noise schedule for our diffusion model. We fix our experiments to 1000 steps with cosine noise schedule~\cite{nichol2021improved}.}
\label{tab:dm_params}
% \vspace{-0.9em}
\centering
\setlength{\tabcolsep}{3pt}
\small
\scalebox{.95}{\begin{tabular}{c|c|c|c}
\toprule
   Noise Schedule & Number of steps & Diversity $(\downarrow)$ & Compatibility $(\downarrow)$\\
    \cmidrule(lr){1-1}\cmidrule(lr){2-2} \cmidrule(lr){3-3} \cmidrule(lr){4-4}
    \multirow{1}{*}{Linear}
    & 1000 & 10.5\scalebox{0.8}{$\pm$0.1} & 2.7\scalebox{0.8}{$\pm$0.04}\\
    \midrule
    \multirow{3}{*}{Cosine}
    & 100 & 19.0\scalebox{0.8}{$\pm$0.8} & 3.1\scalebox{0.8}{$\pm$0.0}\\
    & 1000 & 9.5\scalebox{0.8}{$\pm$0.1} & 2.5\scalebox{0.8}{$\pm$0.0}\\
    & 4000 & 12.0\scalebox{0.8}{$\pm$0.3} & 3.2\scalebox{0.8}{$\pm$0.03}\\
    \bottomrule
\end{tabular}}
\end{table}

%%%%%%
\section{Non-Manhattan RPLAN}
\label{sec:non_manhattan_rplan}
To further evaluate our method, we create a non-manhattan version of RPLAN by randomly adding two additional corners to an outer edge of a floorplan. Concretely, for each room in the house, we break the wall with the highest distance from the center of the house. We instead add two additional corners with a random distance from the center of the room in one axis and center of the wall in the other axis of 2D coordinates. We keep the new corners with a probability of $50\%$ if they do not cause an overlap with the other rooms of the house. Figure~\ref{fig:non_manhattan_samples} shows examples of our non-manhattan version of RPLAN.
\begin{figure}[tb]
    \centering
    \includegraphics[width=0.9\linewidth]{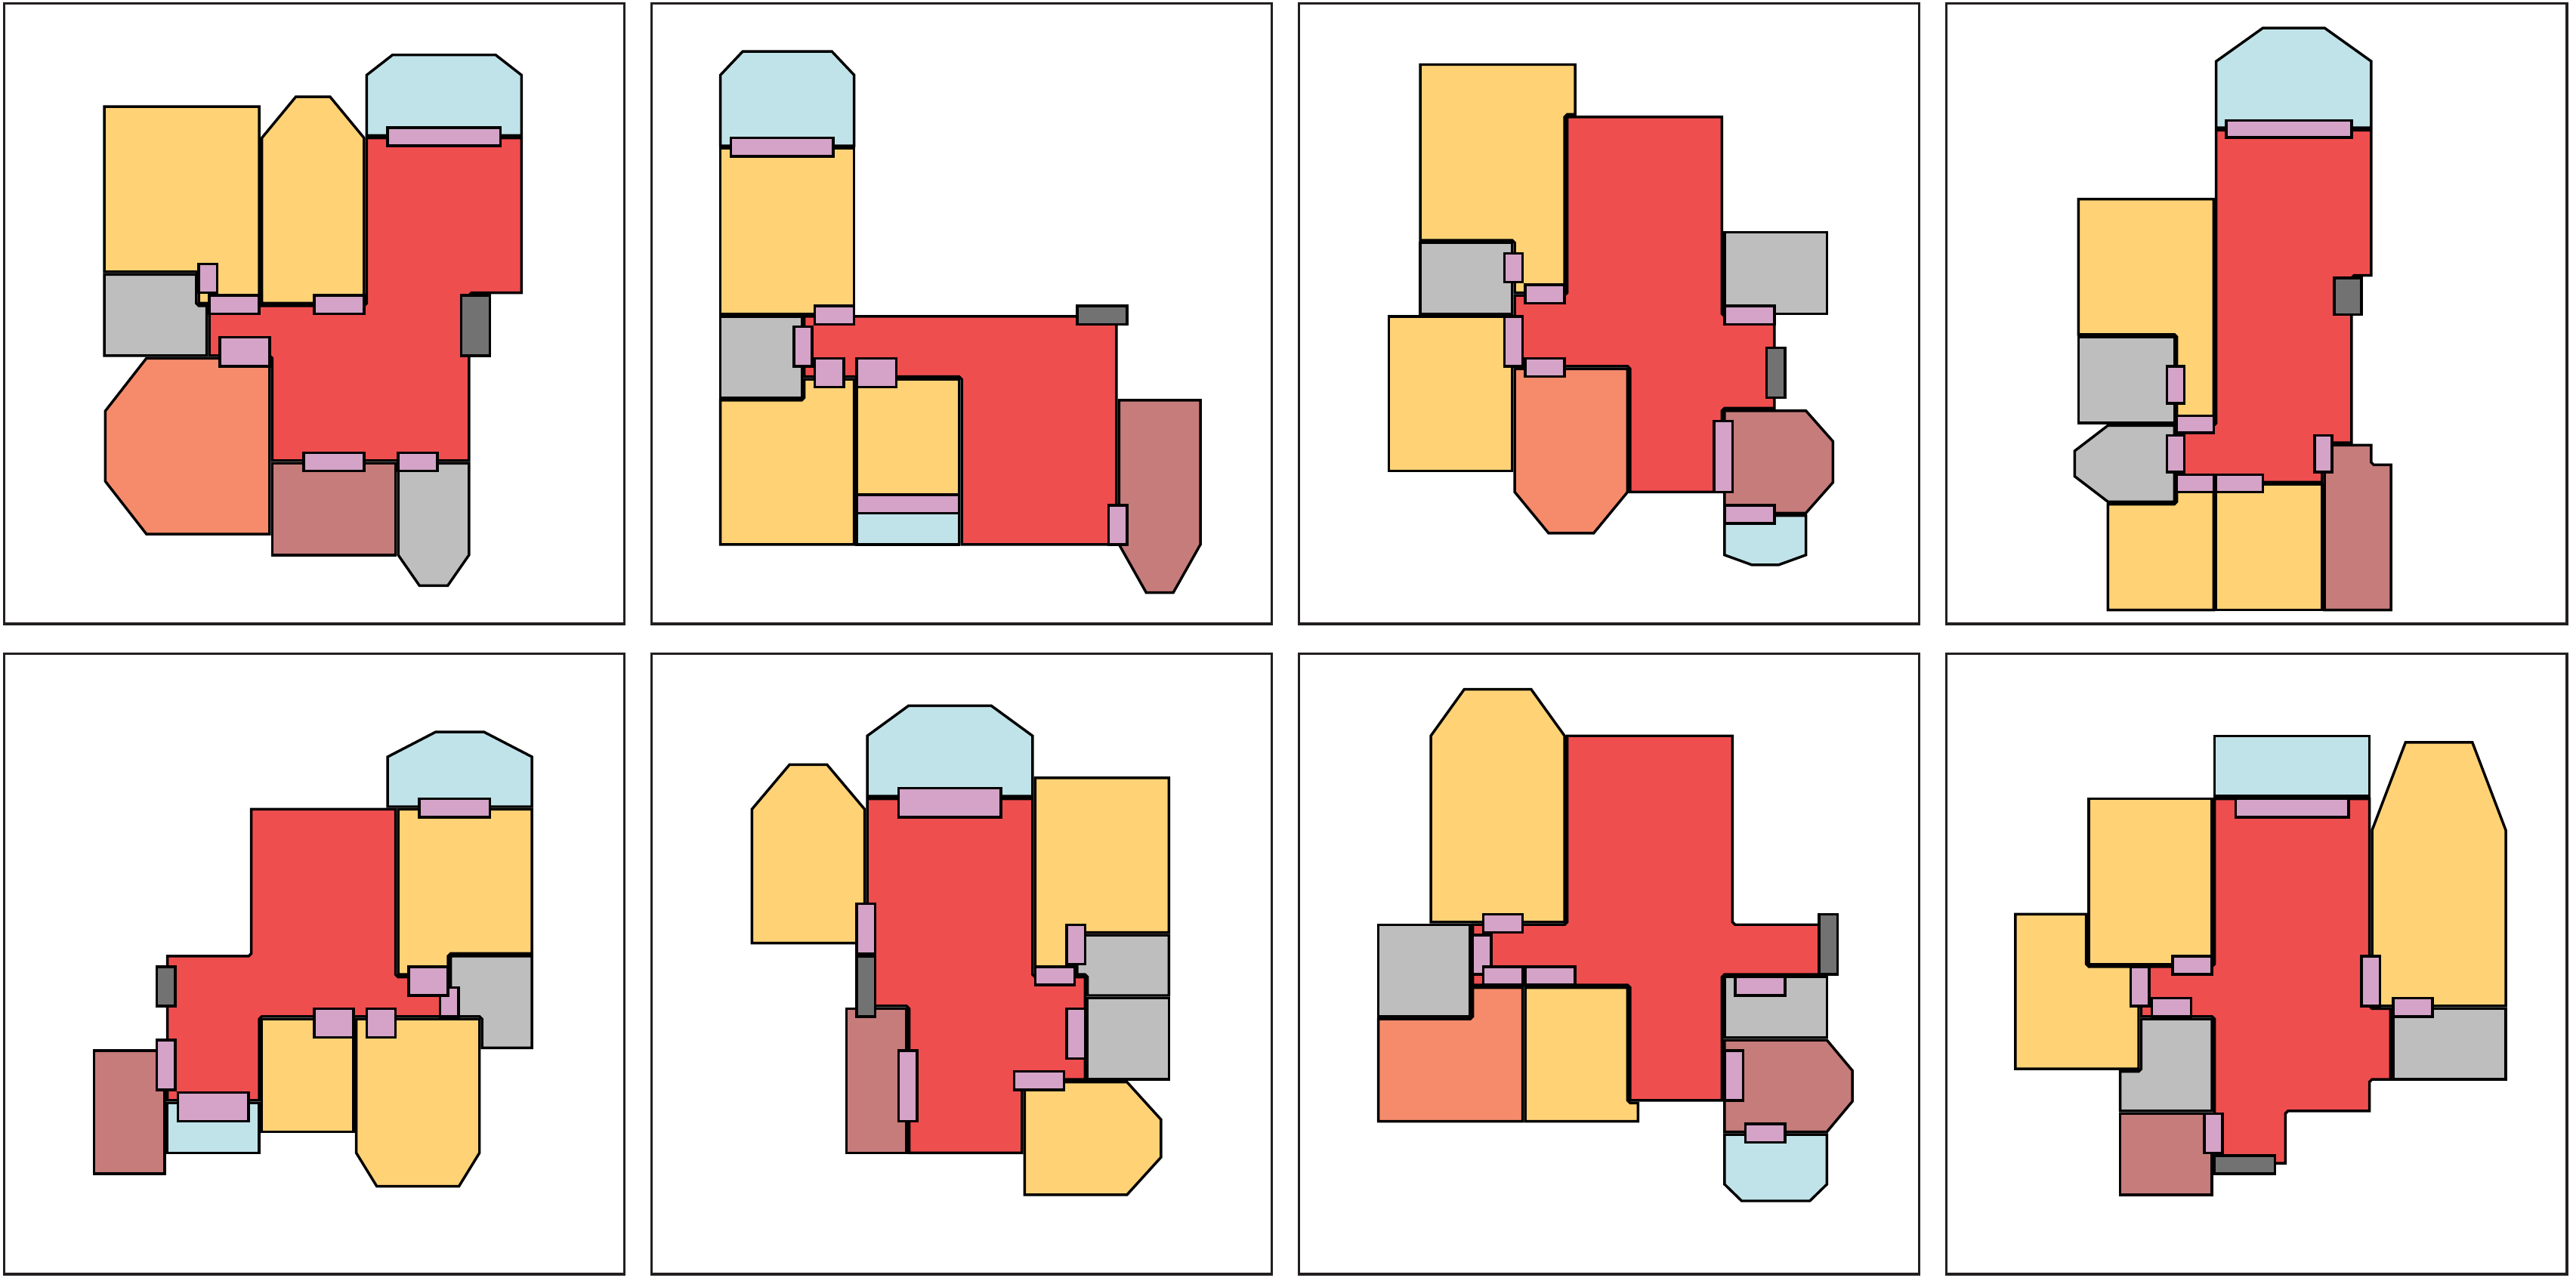}
    \caption{Examples of the created non-manhattan RPLAN dataset.}
    \label{fig:non_manhattan_samples} 
    \vspace{-.5cm}
\end{figure}
%%%%%%
\begin{figure*}
    \centering
    \includegraphics[width=\textwidth]{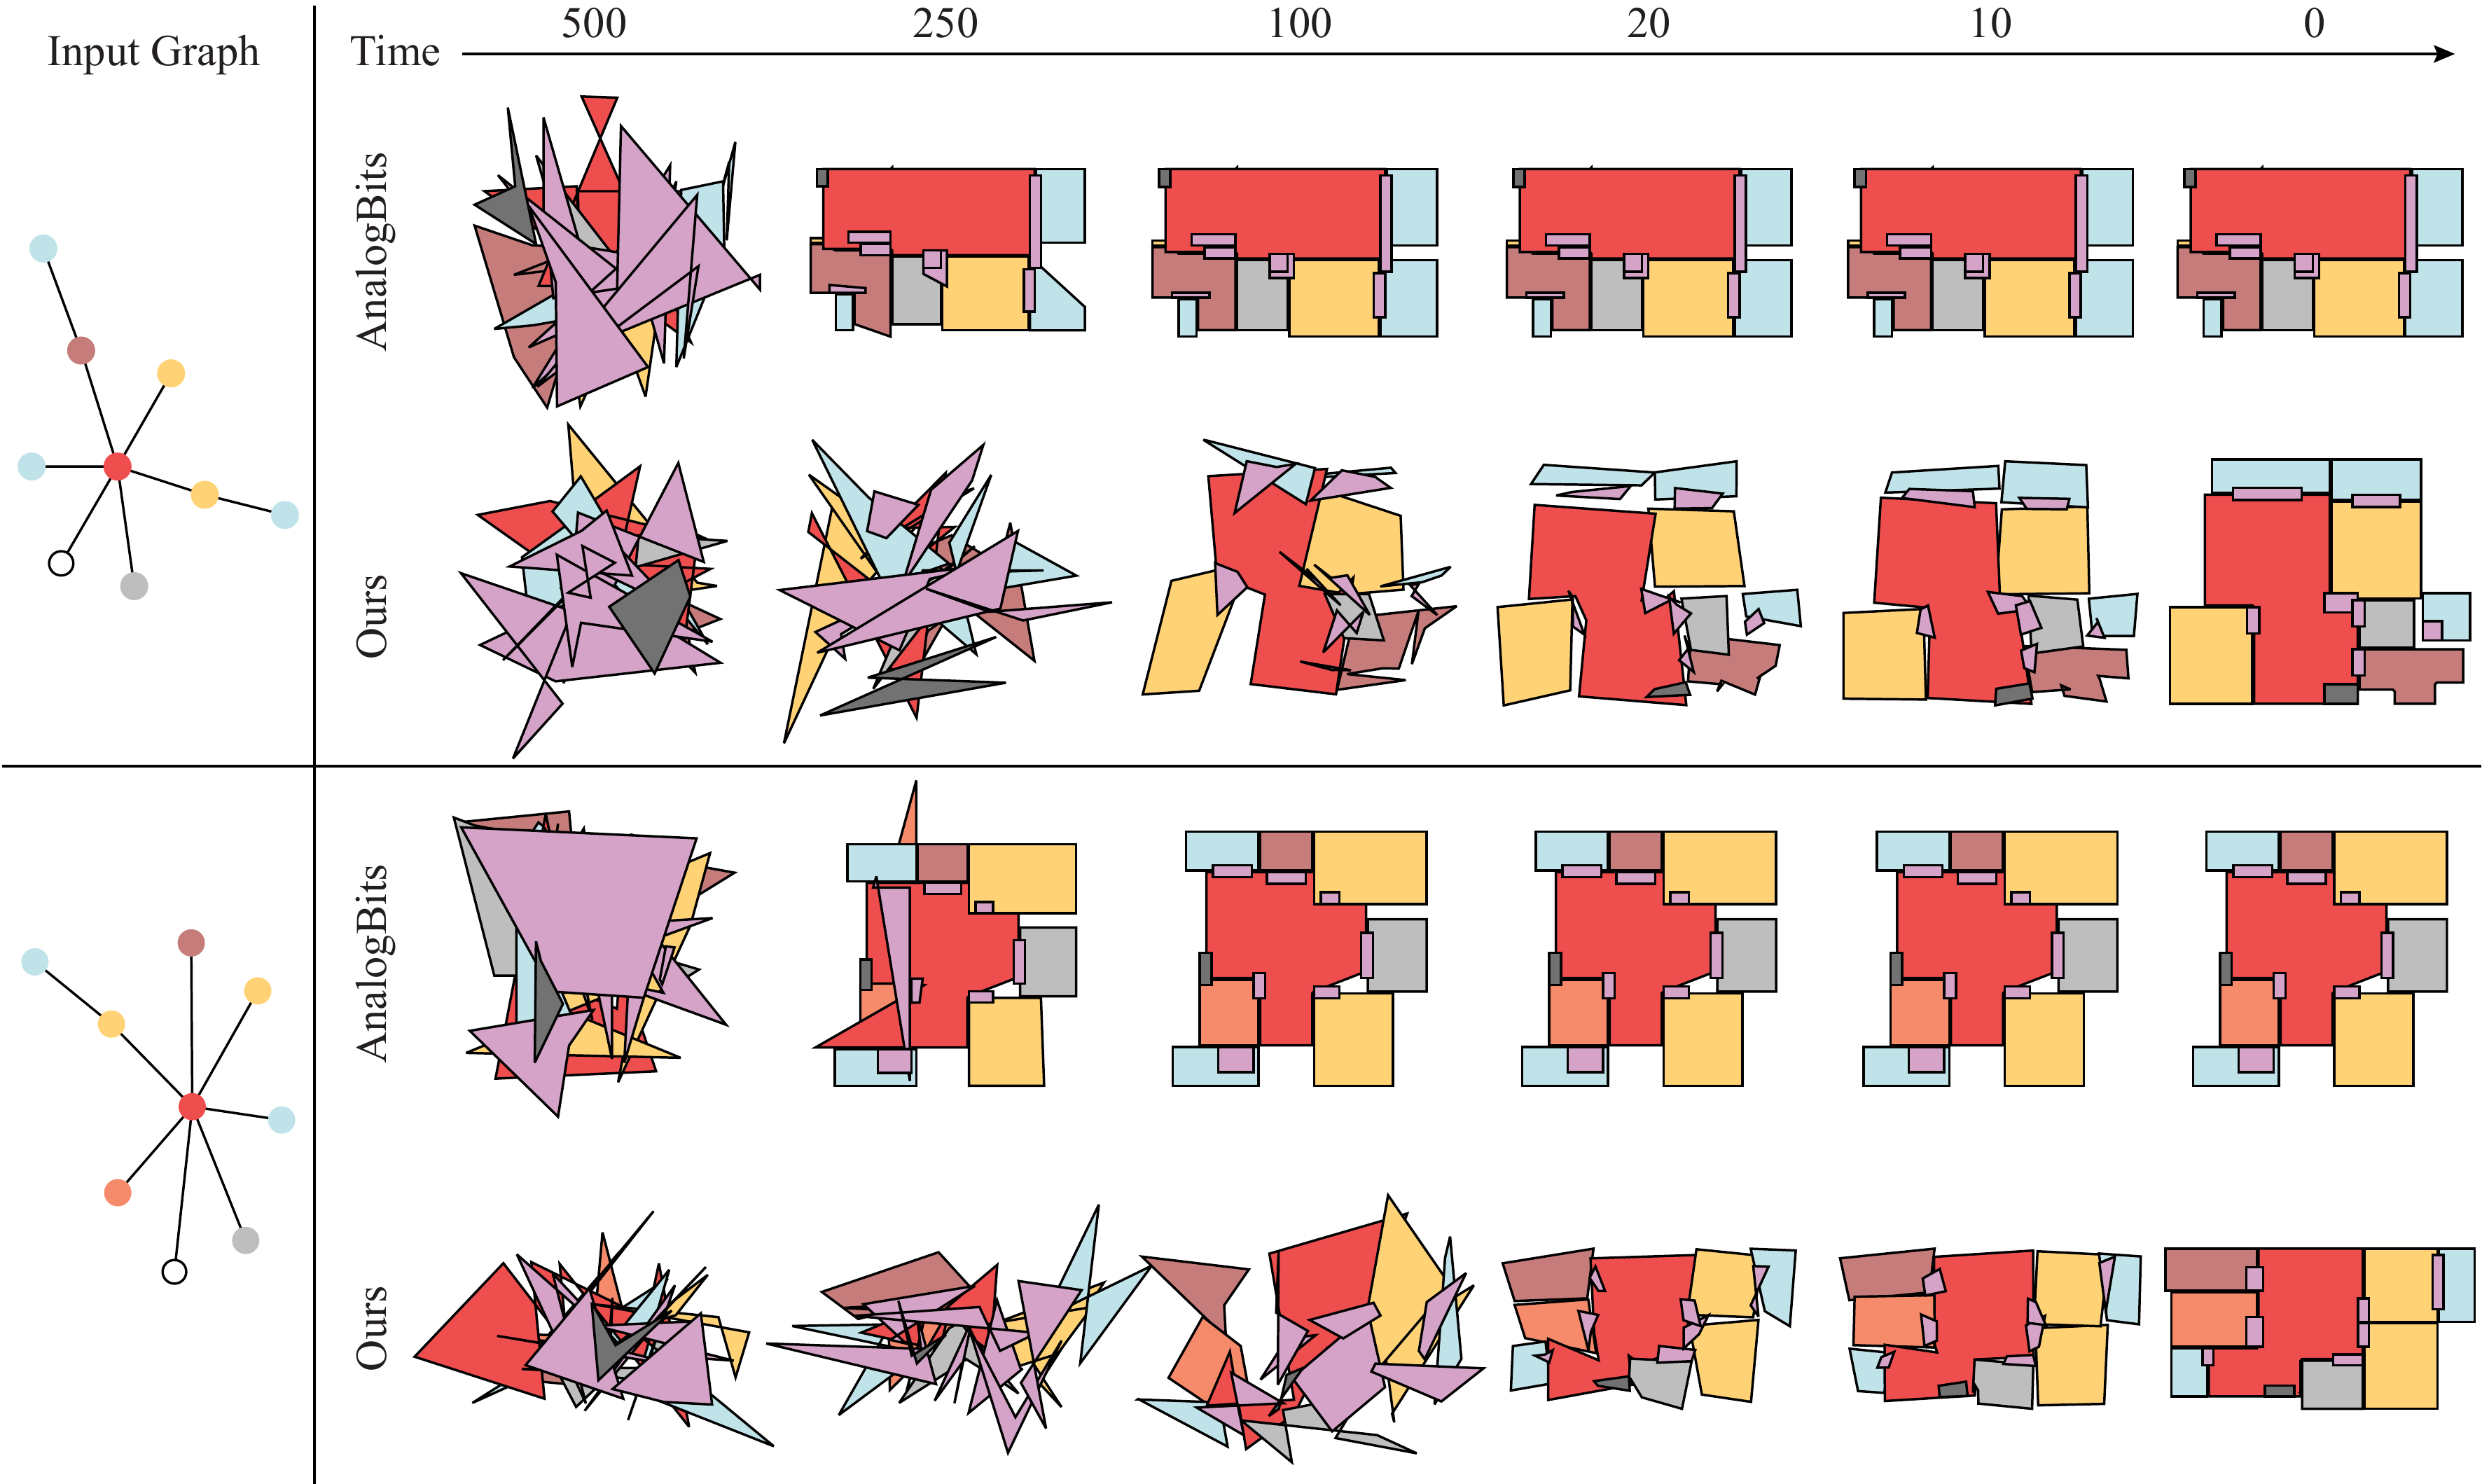}
    \caption{Comparison of our continuous and discrete denoising with AnalogBits based on a given bubble diagram. Our method benefits from all of the steps to refine the generated floorplan while AnalogBits has almost no changes on the final prediction in at least the last 100 steps meaning that the network predicts a simple mapping of input values to 0 and 1 based on a threshold.}
    \label{fig:analog_bits_steps}
\end{figure*}
\begin{figure*}
    \centering
    \includegraphics[width=\textwidth]{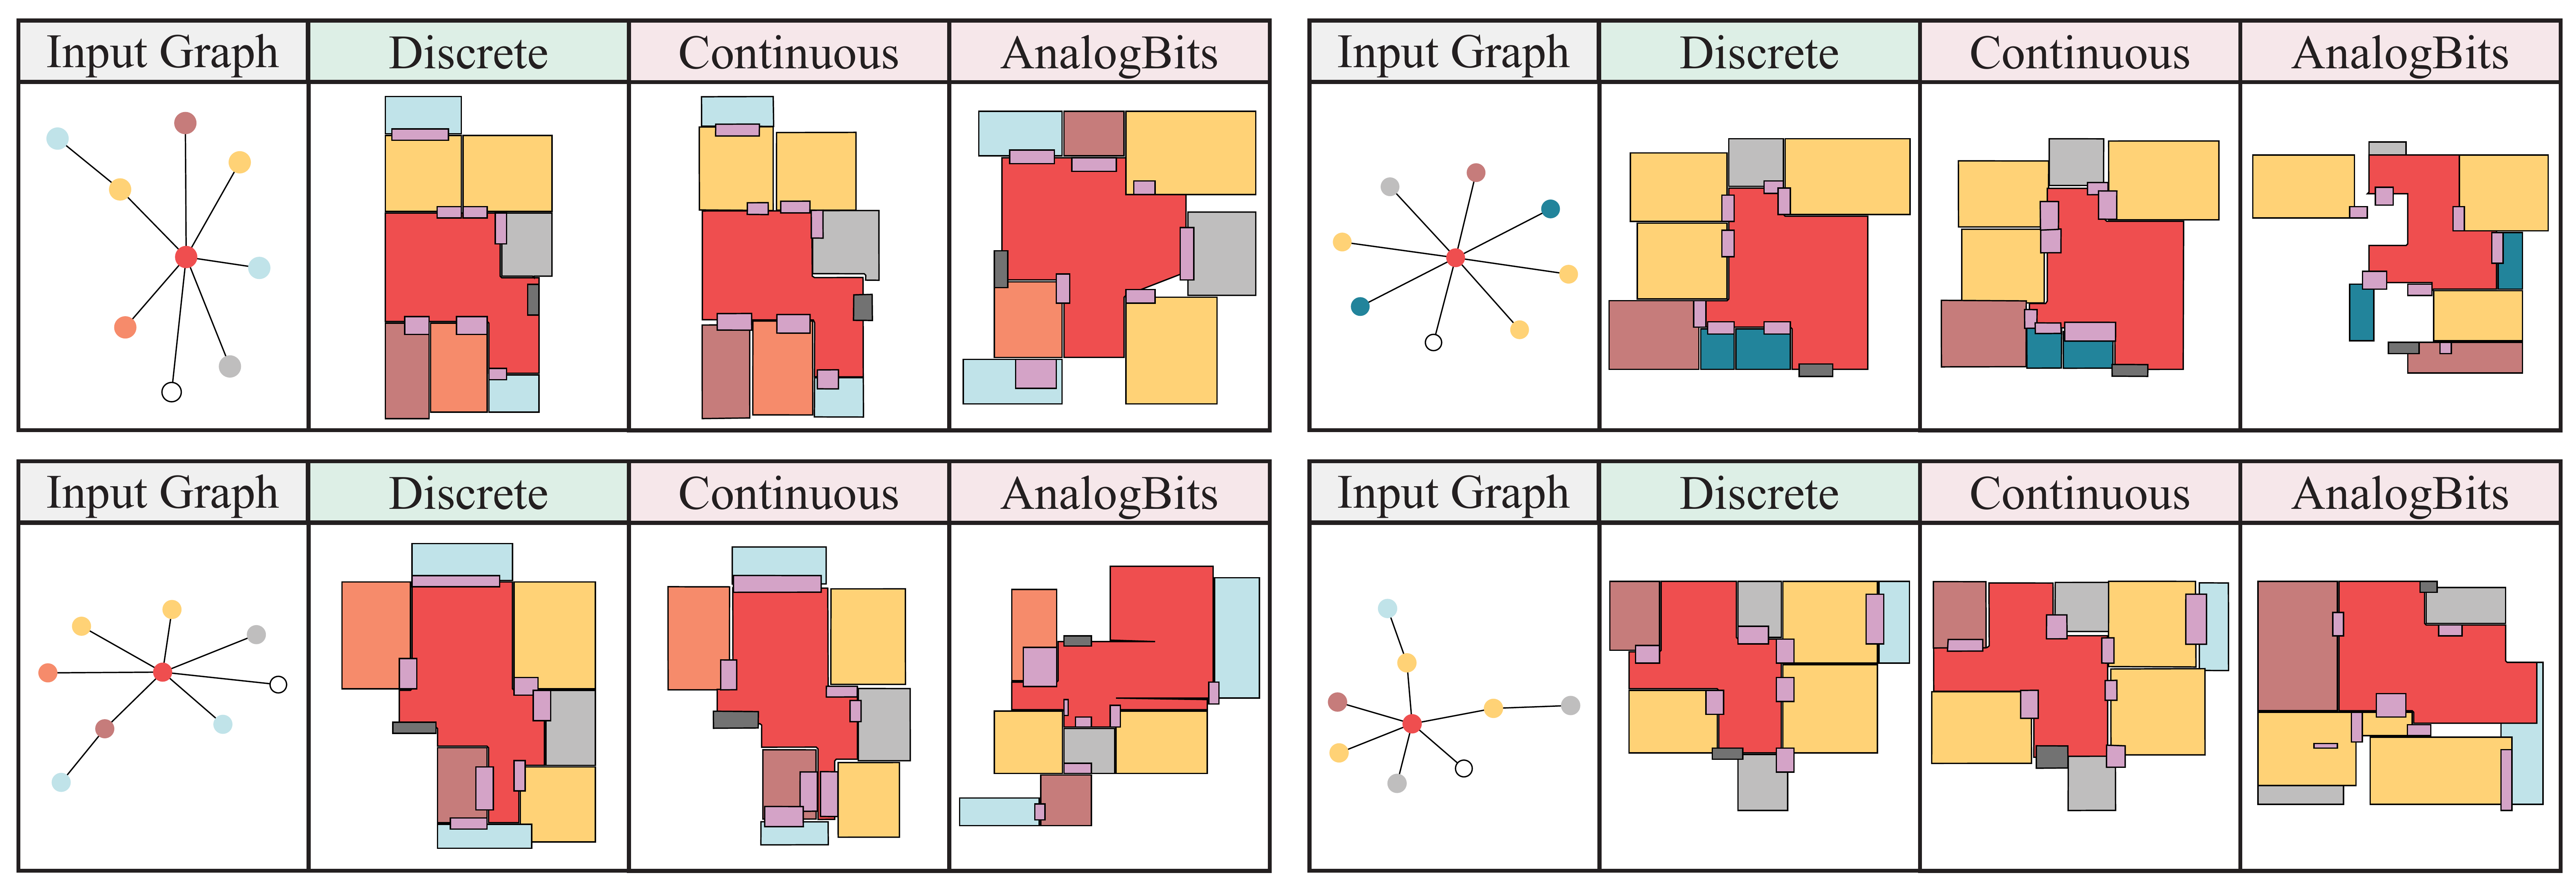}
    \caption{Additional comparison of generated floorplans by our method in both discrete and continuous denoising compared with the results of using AnalogBits for our model. While the results of AnalogBits have significantly lower quality, our model gets high-quality results in continuous head, and the discrete head further improves the results to provide a precise location for each corner.}
    \label{fig:qualitative_analogbits}
\end{figure*}
\begin{figure*}
    \centering
    \includegraphics[width=\textwidth]{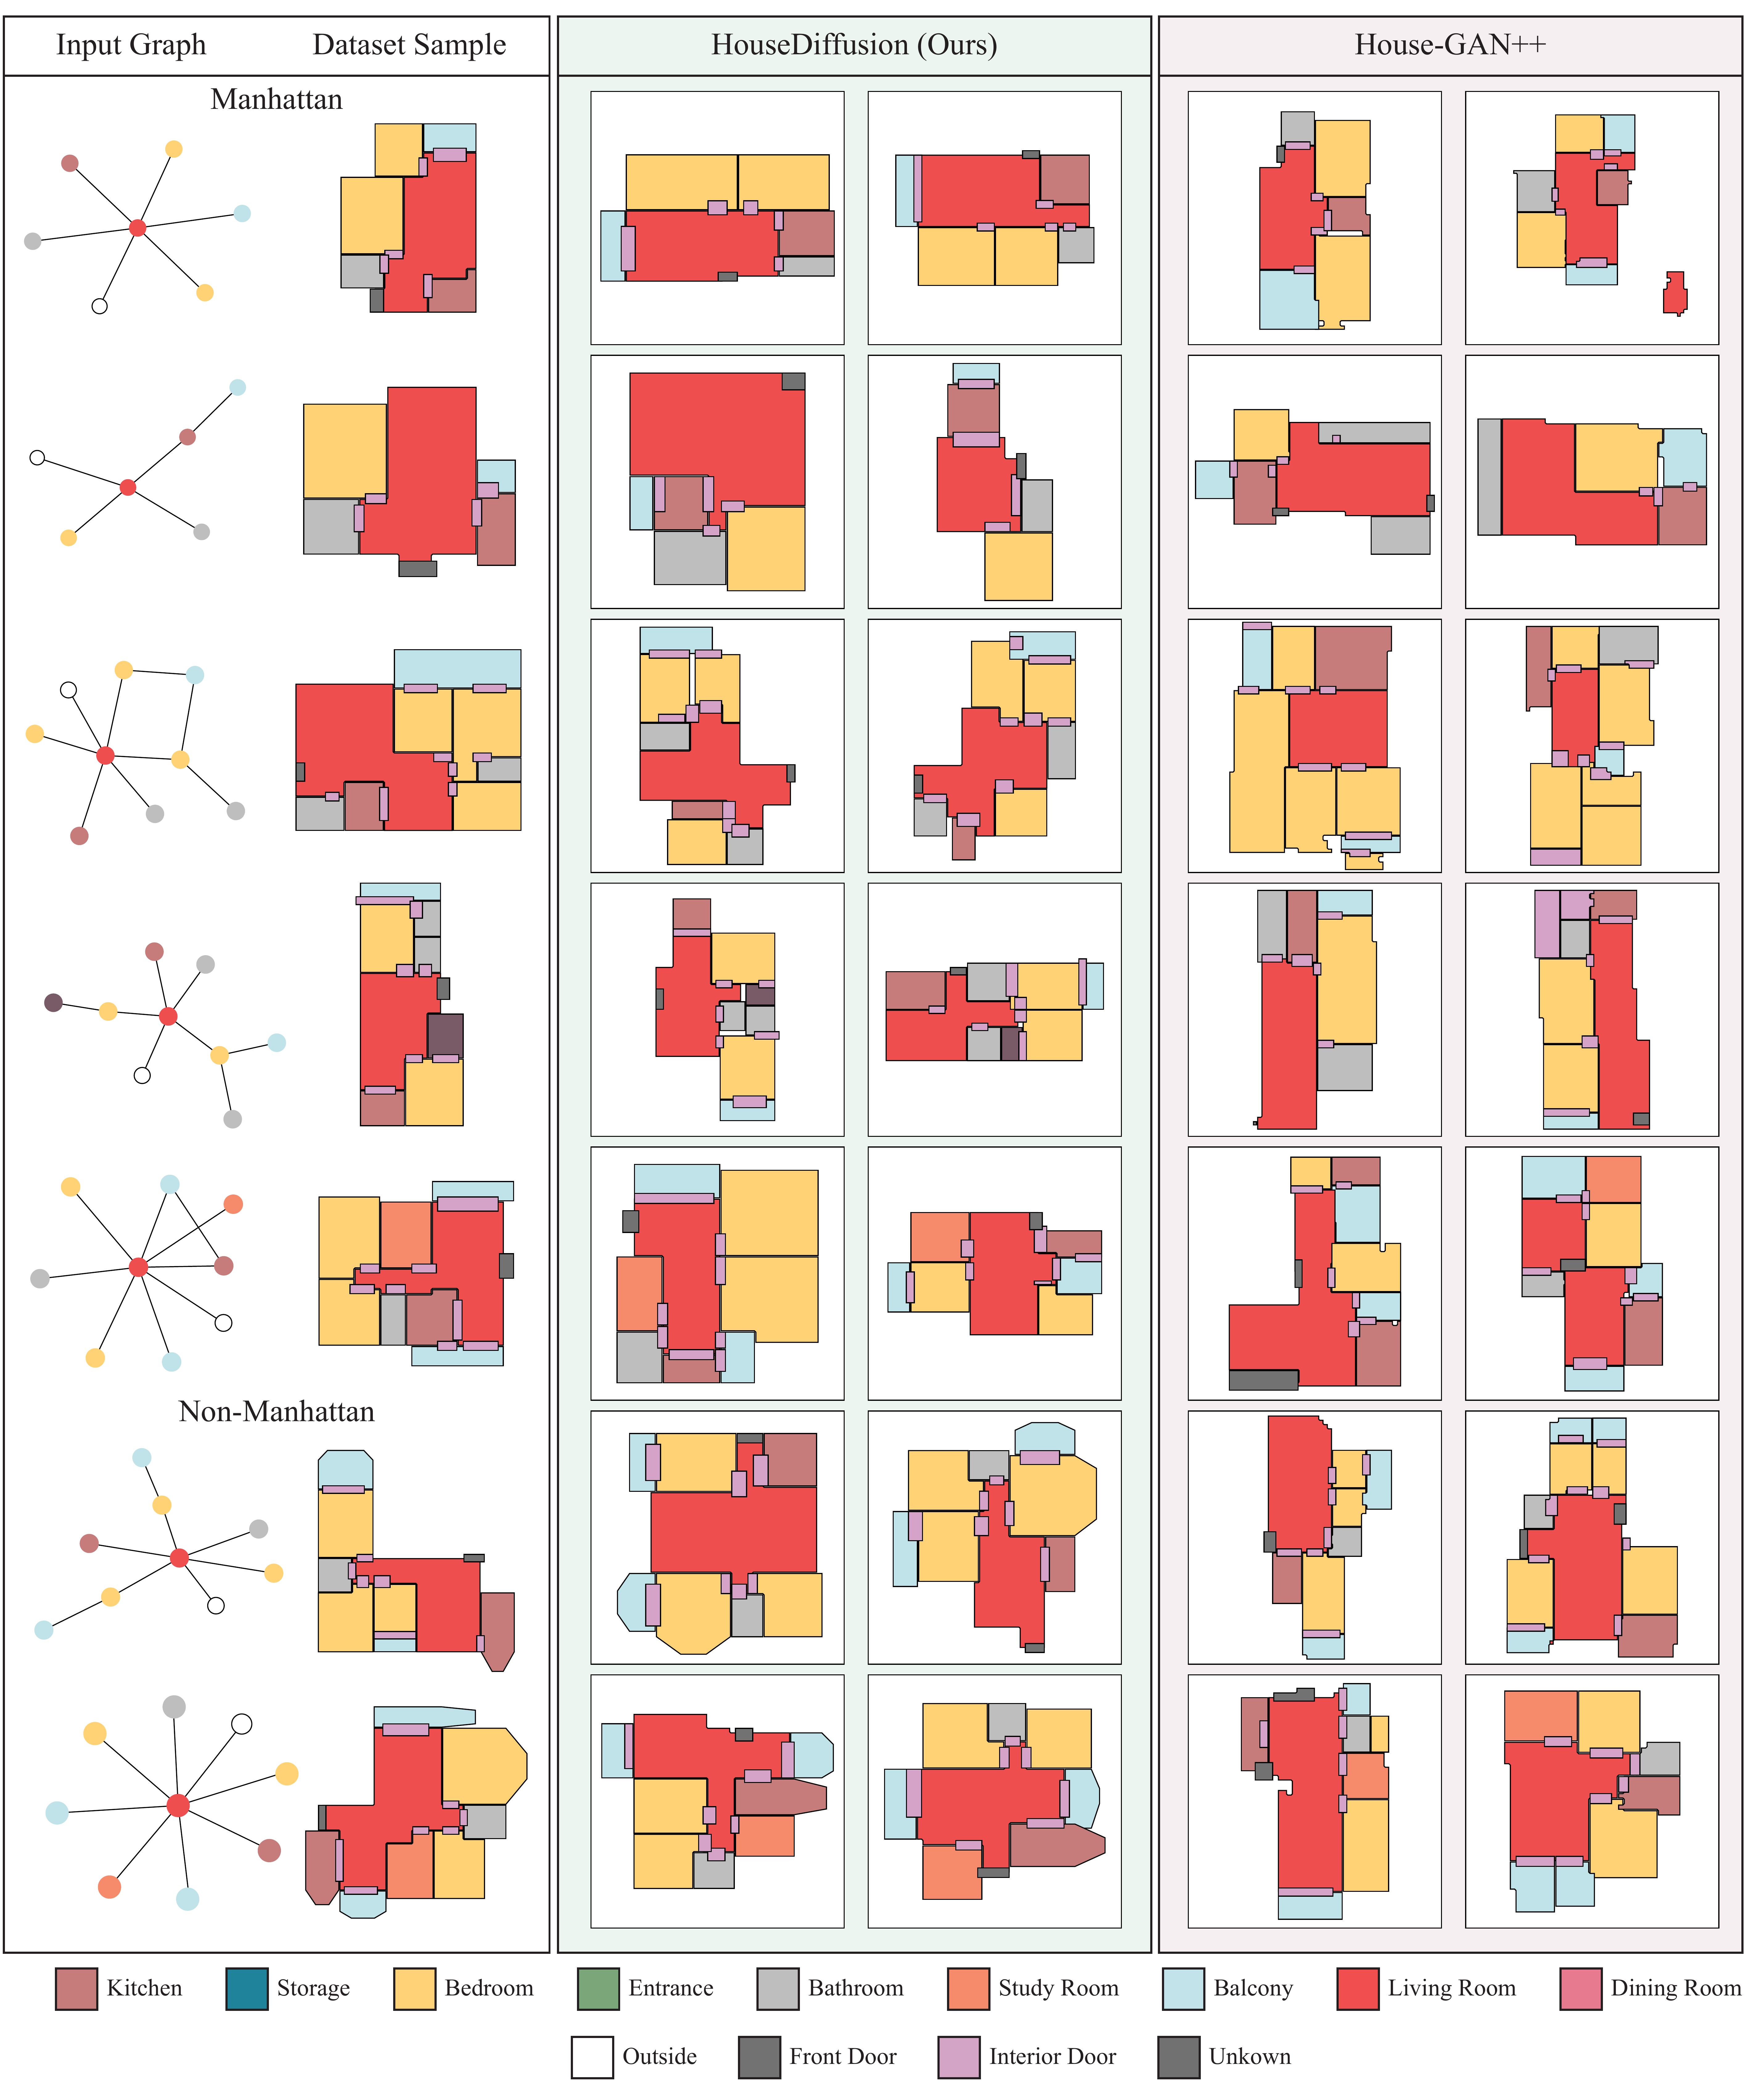}
    \caption{Additional generated floorplan samples against House-GAN++~\cite{houseganpp}. Our results look more diverse and higher quality, where the major issue of House-GAN++ is duplicate or missing rooms, ignoring the input constraint.}
    \label{fig:diversity_comparison_supp}
\end{figure*}

% \newpage~\newpage~\newpage
%%%%%%
\section{Analysis of AnalogBits}
\label{sec:analog_bits}
Chen \etal~\cite{chen2022analog} proposed AnalogBits which directly uses the continuous formulation of diffusion models to denoise a random Gaussian sample to binary values (-1 and 1 in practice) and convert them directly to discrete values by simple thresholding. In Figure~\ref{fig:analog_bits_steps} we visualized different steps of the denoising process obtained by the formulation of AnalogBits compared to our continuous and discrete denoising. We visualize the intermediate steps by considering them as the final output (i.e., using thresholding and binary-to-decimal mapping). The generated floorplans of AnalogBits are roughly the same in the last 100 steps, while our method uses every step to continuously denoise the generated floorplan. We hypothesize that in the case of AnalogBits, when the noise coefficient $\sqrt{(1-\gamma_t)}$ is small (See Equation 1 in the main paper), the network learns a simple mapping of $f:x_t\rightarrow \lfloor x_t+\frac{1}{2} \rfloor$ instead of the dataset distribution, which reduces the final quality of the generated samples.
%%%%%%
% \section{User Study}
% \section{Failure Cases}
%%%%%%

\section{Qualitative Examples}
\label{sec:qualitative_examples}
Figure~\ref{fig:qualitative_analogbits} shows additional comparison of our method with AnalogBits and both continuous and discrete outputs of our model. In addition, we have provided more examples of generated floorplans by our method versus the results of House-GAN++~\cite{houseganpp} in Figure~\ref{fig:diversity_comparison_supp}. Please see the provided video in the supplementary for better visualization of the reverse process of our method as well as additional examples.
